# Supplementary material for: Unison: Benchmarking Unified Multimodal Models via Synergistic Understanding and Generation
Source: arXiv:2606.26984 source file (2026-06-25)
Supplement: Supplementary file 1 [file X_suppl.tex]

\clearpage
\setcounter{page}{1}
%\maketitlesupplementary

\section{Details of Unison Dataset}

\subsection{Details of Dataset Statistic}

\section{Details of Unison Pipeline}
\label{appendix:pipeline}

\section{Qualitative Analysis}
